# Supplementary material for: Uncertainty-aware Cardinality Estimation by Neural Network Gaussian Process
Source: arXiv:2107.08706 source file (2021-07-19)
Supplement: Supplementary file 1 [file appendix.tex]

%\section*{Appendix}

\begin{table}[h]
%\begin{small}
\begin{footnotesize}
%\vspace{-2ex}
% \begin{minipage}[c]{5cm}
\begin{minipage}[t]{2.4cm}
\begin{center}
\begin{tabular}{|l|l|l|} \hline 
$F$ & $T$ & $ew$ \\ \hline \hline
1 & 1 & $a_{11}$ \\ \hline
1 & 2 & $a_{12}$ \\ \hline
2 & 1 & $a_{21}$ \\ \hline
2 & 2 & $a_{22}$ \\ \hline
\end{tabular} \\
\vspace*{0.2cm}
(a) Relation $A$
\vspace*{0.2cm}
\end{center}
\end{minipage}
\quad
\begin{minipage}[t]{2.4cm}
\begin{center}
\begin{tabular}{|l|l|l|} \hline 
\multirow{2}{*}{$F$} & \multicolumn{2}{|c|}{B} \\ \cline{2-3} 
                                & $T$ & $ew$ \\ \hline \hline
\multirow{2}{*}{1}     & 1 & $a_{11}$ \\ \cline{2-3}
                                & 2 & $a_{12}$ \\ \hline
\multirow{2}{*}{2}     & 1 & $a_{21}$ \\ \cline{2-3}
                                & 2 & $a_{22}$ \\ \hline
\end{tabular} \\
\vspace*{0.2cm}
(b) Nested Relation $\NestOp_{(T, ew)\rightarrow B}(A)$
\vspace*{0.2cm}
\end{center}
\end{minipage}
\quad
\begin{minipage}[t]{2cm}
\begin{center}
\begin{tabular}{|c|c|} \hline 
$\TID$ & $vw$ \\ \hline \hline
1 & $c_1$ \\ \hline
2 & $c_2$ \\ \hline
\end{tabular} \\
\vspace*{0.2cm}
(c) Relation $C$
\vspace*{0.2cm}
\end{center}
\end{minipage}
\centering
%\vspace*{-3ex}
\caption{The relation representations}
\label{tbl:rels}
%\end{small}
\end{footnotesize}
% \vspace*{-0.4cm}
\end{table}

\begin{table*}[t]
{\scriptsize
\centering
\begin{minipage}{0.48\linewidth}
%\begin{subtable}
{%\scriptsize
\centering
\begin{tabular}{|l|r|r|r|r|} \hline
   \multirow{2}{*}{\bf \WCC} & \multicolumn{2}{|c|}{\bf \SQL}  & \multicolumn{2}{|c|}{\bf Graph}\\ \cline{2-5} 
   				    & Exe. Time (s) & Shuffle (GB) & Exe. Time (s) & Shuffle (GB) \\ \hline \hline
    \kw{CA}  & 998 & 16.9/29.4 &114  & 2.8/3.7   \\ \hline
    \kw{OK} & 200 & 54.9/37.4 & 56 & 3.3/3.2   \\ \hline
    \kw{AR}  & 2318 & 926.4/581.6 & 287 & 13.5/14.2   \\ \hline
    \end{tabular}
%\end{center}
%\caption{\SQL \& Graph Workflow for \WCC for 9 Intances}
\caption{\WCC for 9 Instances}
\label{tbl:sql2graph:wcc9}
%\end{center}
}
\end{minipage}
\vspace*{-0.3cm}
%
%\vspace*{-0.3cm}
%\begin{subtable}
\begin{minipage}{0.48\linewidth}
{%\scriptsize
\centering
\begin{tabular}{|l|r|r|r|r|} \hline
   \multirow{2}{*}{\bf \SSSP} & \multicolumn{2}{|c|}{\bf \SQL}  & \multicolumn{2}{|c|}{\bf Graph}\\ \cline{2-5} 
   				    & Exe. Time (s) & Shuffle (GB) & Exe. Time (s) & Shuffle (GB) \\ \hline \hline
    \kw{CA}  & 638 & 17.6/22.9 & 78 & 0.226/0.302   \\ \hline
    \kw{OK} & 272 & 54.7/38 & 50 & 2.3/2.2   \\ \hline
    \kw{AR}  & 2,858 & 249.7/189.8 & 281 & 6.3/6.6   \\ \hline
    \end{tabular}
%    \caption{\SQL \& Graph Workflow for \SSSP  for 9 Intances}
\caption{\SSSP  for 9 Instances}
\label{tbl:sql2graph:sssp9}
%\end{center}
}
\end{minipage}
%\vspace*{-0.3cm}
%
%
\begin{minipage}{0.48\linewidth}
%\begin{subtable}
{%\scriptsize
\centering
\begin{tabular}{|l|r|r|r|r|} \hline
   \multirow{2}{*}{\bf \PR} & \multicolumn{2}{|c|}{\bf \SQL}  & \multicolumn{2}{|c|}{\bf Graph}\\ \cline{2-5} 
   				    & Exe. Time (s) & Shuffle (GB) & Exe. Time (s) & Shuffle (GB) \\ \hline \hline
    \kw{CA}  & 152 & 4.2/6.7 & 72 & 1.5/1.6   \\ \hline
    \kw{OK} & 758 & 104.9/84.9 & 152 & 9/9.3   \\ \hline
    \kw{AR}  & 1,358 & 787.6/551.3 & 419 & 28.1/31.2   \\ \hline
    \end{tabular}
%    \caption{\SQL \& Graph Workflow for \PR  for 9 Intances}
  \caption{\PR  for 9 Instances}
\label{tbl:sql2graph:pr9}
%\end{center}
}
\end{minipage}
\vspace*{-0.3cm}
%
%\vspace*{-0.3cm}
%\begin{subtable}
\begin{minipage}{0.48\linewidth}
{%\scriptsize
\centering
\begin{tabular}{|l|r|r|r|r|} \hline
   \multirow{2}{*}{\bf \LP} & \multicolumn{2}{|c|}{\bf \SQL}  & \multicolumn{2}{|c|}{\bf Graph}\\ \cline{2-5} 
   				    & Exe. Time (s) & Shuffle (GB) & Exe. Time (s) & Shuffle (GB) \\ \hline \hline
    \kw{CA}  & 321 & 7.5/8.3 & 150 & 1.6/3   \\ \hline
    \kw{OK} & 758 & 152.2/129.5 & 524 & 8.3/10.3   \\ \hline
    \kw{AR}  & 1,778 & 454.5/294.6 & 2,071 & 41.9/45.4   \\ \hline
    \end{tabular}
 %   \caption{\SQL \& Graph Workflow for \LP  for 9 Intances}
        \caption{\LP  for 9 Instances}
\label{tbl:sql2graph:lp9}
%\end{center}
}
\end{minipage}
\vspace*{-0.4cm}
\label{tbl:sql2graph9}
}
\end{table*}

\section{{Spark SQL} and {GraphX} on {Spark}}
\label{app:sec:spark}

\Spark~\cite{DBLP:conf/nsdi/ZahariaCDDMMFSS12} has emerged as the de
facto distributed big data processing system being widely used. It
supports a one-stop resolution for big data-crunching needs by
combining \mapreduce-like capabilities for structured-data processing,
stream processing, machine learning, and graph processing.
The core data abstraction in \Spark is \RDD (Resilient Distributed
Dataset), which is an immutable in-memory abstraction to be
partitioned and computed on a cluster in a fault-tolerant manner.
A driver program is written to define {\RDD}s, and an \RDD is
manipulated by two kinds of operation, namely, transformations and
actions. Transformations (e.g. \Map, \Filter) take one or more {\RDD}s
as input to produce a new \RDD, whereas actions (e.g. \Take, \Reduce)
return object data computed from \RDD to the driver program.
%
%%%%%%%%%%%%%%%%%%%%%%%%%%%%%%%%%%%%%%%%%%%%%%%%%%%%%%%%%%%%%%%%%%%%%
% \Spark executes the transformations lazily: a \Spark application does
% not execute until the driver program calls an action.
%
For each action, the \Spark scheduler launches a job and builds an
execution graph using \RDD dependencies. Each job consists of
stages. For each stage, multiple transformations can be pipelined and
divided into a collection of tasks that represent each parallel
computation unit for one partition of the input. Between stages,
\Spark materializes the \RDD and shuffles it among the computational
nodes in the cluster. The efficient \RDD computation builds the
foundation of efficient iterative computation which \Hadoop falls
down.
On top of \Spark, there are two systems, \Spark~\SQL and \GraphX, that
are most related to our work.

\stitle{Spark SQL}: \Spark~\SQL~\cite{ArmbrustXLHLBMK15}, originated
from {\sl Shark}~\cite{DBLP:conf/sigmod/XinRZFSS13}, is a structured
data processing module on \Spark. \Spark~\SQL provides
high-performance in-memory relational processing by \rdbms techniques
with the support of \SQL'92 syntax.  Note that \Spark~\SQL does not
support any recursive \SQL queries as specified in \SQL'99.
For a user-given \SQL query, the parser builds an unresolved logical
plan composed of logical operators~(e.g. join, aggregate, etc.). The
analyzer looks up meta-data from the catalog and resolves the logical
plan by a collection of analyzing rules. The logical plan is further
transformed by both rule-based and cost-based optimizations. In the
physical planning phase, the optimized logical plan is transformed to
physical plans by a collection of strategies. A physical plan is
composed of physical operators~(e.g. ShuffleHashJoin, BroadcastJoin,
etc.), which are implemented by the basic operations on \RDD with row
type.
The core component of \Spark~\SQL is the \Catalyst optimizer. It takes
an unresolved logical plan and returns an optimized logical
plan. \Catalyst groups optimization rules into batches, and explores
batches until the logical plan reaches a fixpoint. \Catalyst is
highly extensible for developers.
%
% The existing cost model is simple
% and is mainly used for join reordering and selecting a physical join
% operator.

\stitle{GraphX}: \GraphX~\cite{DBLP:journals/corr/XinCDGFS14} is an
embedded graph processing framework built on top of \Spark. It
represents graph-structured data as a property graph, where each
vertex/edge is associated with attributes. Like \RDD, the internal
abstraction of the property graph, \gdata, is immutable, distributed,
and fault tolerant. The \gdata is logically equivalent to a pair of
special {\RDD}s. One is \VertexRDD, for a collection of vertices,
represented by key-value pairs, where the key is a unique id and
value is typed attributes. The other is \EdgeRDD, for a collection of
edges, represented by triples of (\SrcId, \Attr, \DstId) for directed
edges from \SrcId to \DstId associated with value \Attr.

To support graph algorithms, \GraphX extends \Spark operations with a
collection of operators that take functions as parameters and produce
new \gdata. Based on functionality, these operators are classified
into 4 main categories: (1) Property Operators, (2) Structural
Operators, (3) Join Operators and (4) Neighborhood Aggregation. In
addition, as the \VertexRDD and \EdgeRDD are two special {\RDD}s with
optimized data structures, \GraphX provides extra efficient operations
for them respectively. Such operations can take advantage of the
optimized data structures and indices, besides the general \RDD
transformations.

In addition, \GraphX supports custom iterative graph algorithms by the
\PregelAPI API. The implementation of \PregelAPI is inspired by
Google's \Pregel so that it is based on Bulk Synchronous Parallel
(\bsp) model. For \PregelAPI, each iteration is a
superstep. Between consecutive iterations, the synchronization
barrier synchronizes messages shuffling among the computational nodes
in the cluster. Many of \GraphX built-in graph algorithms
(e.g. \PageRank)
% , \ConnectedC)
are implemented by a single \PregelAPI call.

\section{Some Proofs}
\label{app:proof}
\stitle{The proof sketch of the $\Rule_{NA}$ rule in
  Eq.~(\ref{eq:nested:agg-join})}:  
% \begin{proof}
For any flat relation $R$ and $R_N = \NestOp_{(B_1,\cdots, B_m)
  \rightarrow B }(R)$, we have
\begin{equation}
\label{eq:nested:agg-join:1}
\sigma_{A = a}( _{A}\mathcal{G}_{\mathring{f}}(R)) = \mathcal{G}_{\mathring{f}}( (\sigma_{A = a} R_N).{B} )
\end{equation}
satisfied for $\mathring{f}(B) = \mathring{f}(B_1, \cdots, B_m)$.
 
 For $\forall a$ with non-null value, we have 
 
 \begin{equation}
\begin{split}
\displaystyle{ \sigma_{A= a} (_{A}\mathcal{G}_{\mathring{g}} ( \rho_{R_1}(_{A}\mathcal{G}_{\mathring{f}~\kw{as}~fv}(R) )\mathop{\Join}_{\substack{R_1.A = R.A \\ R_1.fv = R.B_i} } R ))}
=  \\
\displaystyle{ \mathcal{G}_{\mathring{g}} ( \rho_{R_1}( \sigma_{A =a}(_{A}\mathcal{G}_{\mathring{f}~\kw{as}~fv}(R) ))\mathop{\Join}_{\substack{ R_1.fv = R.B_i} }  \sigma_{A=a} (R) )}
\label{eq:nested:agg-join:2}
\end{split}
\end{equation}
satisfied as the selection $\sigma_{A=a}$ is pushed down into the equi-join. By applying Eq.~(\ref{eq:nested:agg-join:1}) to Eq.~(\ref{eq:nested:agg-join:2}). We have Eq.~(\ref{eq:nested:agg-join:2}) equals to 

\begin{equation}
\displaystyle{ \mathcal{G}_{\mathring{g}}( ( \rho_{R_1}( \mathcal{G}_{\mathring{f}}( \sigma_{A = a} (R_N).{B} ) )~\kw{as}~fv)\mathop{\Join}_{\substack{ R_1.fv = R.B_i} }  \sigma_{A=a} (R) )}
\label{eq:nested:agg-join:3}
\end{equation}
The equi-join on $R.B_i$ of  $\sigma_{A = a}(R)$ is equivalent to equi-join of on the sub-relation $\sigma_{A=a}(R.B)$ on the column $B.B_i$. Therefore, Eq.~(\ref{eq:nested:agg-join:3}) equals to 
\begin{equation}
\displaystyle{ \mathcal{G}_{\mathring{g}}( ( \rho_{R_1}( \mathcal{G}_{\mathring{f}}( \sigma_{A = a} (R_N).{B} ) )~\kw{as}~fv)\mathop{\Join}_{\substack{ R_1.fv = {B}.B_i} }  \sigma_{A=a} ( \mu_{B}(R_N) ) )}
\label{eq:nested:agg-join:4}
\end{equation}
By assigning the $R_1.fv$ to $_{A}\mathcal{G}_{\mathring{f}~\kw{as}~fv}(R)$, we have Eq.~\ref{eq:nested:agg-join:4} is equal to Eq.~(\ref{eq:nested:agg-join:5}) where the equi-join is avoid.
\begin{equation}
\displaystyle{ \mathcal{G}_{\mathring{g}}(  \sigma_{{B}.B_i = \mathcal{G}_{\mathring{f}}( \sigma_{A = a} (R_N).{B} ) } \mu_{B}(\sigma_{A=a}(R_N) ) )}
\label{eq:nested:agg-join:5}
\end{equation}
And Eq.~(\ref{eq:nested:agg-join:5}) is equal to Eq.~(\ref{eq:nested:agg-join:6})
\begin{equation}
\displaystyle{\sigma_{A = a}  (\mathcal{G}_{\mathring{g}}(  \sigma_{{B}.B_i = \mathcal{G}_{\mathring{f}}( R_N.{B} ) } \mu_{B}(R_N ) ))}
\label{eq:nested:agg-join:6}
\end{equation}
Since $\mathring{g}$ is an aggregate functions on $(B_1, \cdots, B_m)$, $\mathcal{G}_{\mathring{g}}( \sigma_{B.B_i = \mathcal{G}_{\mathring{f}}} B )$ can be regarded as a projection $\mathcal{F}(B)$ on nested relation $R_N$. Therefore, we have it equals to Eq.(\ref{eq:nested:agg-join:7})
\begin{equation}
\sigma_{A = a} (\UnnestOp_{{B}}(\Pi_{A, \mathcal{F}({B})}(R_N)))
\label{eq:nested:agg-join:7}
\end{equation}
%

%\section{Implementation details in constructing a graph}
\section{Some Implementation details}
\label{app:sec:details}

%We discuss some implementation details in constructing a graph.
%
% Before building a \gdata from the relations get from \rdbms or hdfs,
% our framework access the underlying data to do some checking.
%
We conduct some checkings to further understand the properties of the
graph to be constructed, in order to detect the algebraic
characteristics of the data which helps the physical plan generation
and optimization. We check self-loop and edge direction.  All of the
checkings are composed by several \RDD transformations and actions,
whose cost is negligible comparing to the overall iterative query
processing.
Suppose $r_{E}$ is the \RDD corresponds to the relation $E$. 
For Self-loop checking, it checks if there are any self-loop edges,
$(v, v)$, in the relation $E$ that represent edges.
% 
% let $E(F, T, ew)$ be the relation
% representation for a $n \times n$ matrix \kw{M}, where $F$ and $T$ are
% the two dimension of the matrix. The self-loop checking is to verify
% whether for each $F$( and $T$), there is a tuple $(F, F, *)$( and $(T,
% T, *)$) in the relation $E$.
% In other words, all the diagonal elements of \kw{M} are not \kw{zero}.
%
We check if there are any self-loops by the number of non-zero
diagonal elements in the corresponding matrix representation. In
\GraphX, the number of diagonal elements can be computed by the
operations $r_{E}$.\kw{filter}(\kw{case}$(k,v) => k.\_1 =
k.\_2$).\kw{count}, where conditions can be specified in the
\kw{filter} function to check the value of the diagonal elements.
Note that, in our system, we model a graph as a weighted directed
graph. We check if the graph to be constructed is, in fact, a directed
graph or an undirected graph by edge orientation checking, i.e., if there is an edge $(v, u)$ for an edge $(u, v)$ in the edge
relation. In other words, we check if the corresponding matrix
representation of the edge relation is symmetric.
In \GraphX, the \RDD operation $r_{E}$.\kw{filter}(\kw{case}$(k,v) =>
k.\_1 > k.\_2$).\kw{count} computes the number of elements in the
upper triangular part of a matrix. We can also count the number of
elements in the lower triangular part of a matrix in a similar way.
These checking can be done in an early stage when it is known that it is
possible to use graph-based operators.

\noindent
\underline{Graph Partitioning}: When a graph is built, we explicitly
specify a partition strategy in \GraphX. According to
\cite{pvldb/VermaLSG17}, for \GraphX, the Canonical Random works well
with low degree graphs, and the 2D Edge partitioning works well with
heavy-tail graphs. Here we use the Kurtosis to evaluate the skewness of
the degree distribution~\cite{decarlo1997meaning}, as defined by
Eq.~(\ref{eq:kurtosis}), where $X$ is the random variable denoting the
vertex degree, $\alpha$ and $\sigma$ is its mean and standard deviation, respectively.
\begin{equation}
\displaystyle{ Kurt[X] } = E[( \frac{X- \alpha }{\sigma })^{4}]
= \frac{ E[(X- \alpha)^{4}]}{ (E[(X- \alpha)^{2}])^{2}}
\label{eq:kurtosis}
\end{equation}
If the kurtosis is negative ($Kurt[X] <3$), we adopt the Canonical
Random partitioning. Otherwise, 2D Edge partitioning is chosen. It is
worth mentioning that this statistics can be computed efficiently by
several \RDD transformations. For large graph, we sample a fixed
number of vertex uniformly.

\section{Some Experiments}
\label{app:exp}
\stitle{Varying the scale of cluster}: We test the 4 algorithms on a
smaller cluster of 9 same EC2 instances. Corresponding results are
shown in Table~\ref{tbl:sql2graph:wcc9},
Table~\ref{tbl:sql2graph:sssp9}, Table~\ref{tbl:sql2graph:pr9}, and
Table~\ref{tbl:sql2graph:lp9}, respectively.
We find the executing time increase for both \SQL and graph workflows
when the number of instances decrease in general.  A small dataset,
(e.g. \kw{CA}) runs fast on smaller cluster.
From 16 to 9 instances, the increasing of shuffle size of \kw{AR} in
the \SQL workflow is caused as the total memory size decreases, where
more data to be shuffled is spilled and loaded from disk.
On the other hand, the graph workflow still keeps a stable shuffling
size so that it outperforms the \SQL workflow significantly.
It is worth mentioning that, for \LP on \kw{AR}, the graph workflow
spends a longer executing time than that of the \SQL workflow due to
over 40\% time of garbage collection. This is because \gdata takes
more memory than \RDD and the memory available has a great influence
on the performance \Spark.

\comment{
\begin{equation}
\begin{split}
\displaystyle{ \sigma_{A= a} (_{A}\mathcal{G}_{\mathring{g}} ( \rho_{R_1}(_{A}\mathcal{G}_{\mathring{f}~\kw{as}~fv}(R) )\mathop{\Join}_{\substack{R_1.A = R.A \\ R_1.fv = R.B_i} } R ))}
\Leftrightarrow  \\
\displaystyle{ (\mathcal{G}_{\mathring{g}} ( \rho_{R_1}( \sigma_{A =a}(_{A}\mathcal{G}_{\mathring{f}~\kw{as}~fv}(R) ))\mathop{\Join}_{\substack{ R_1.fv = R.B_i} }  \sigma_{A=a} (R) ))}
\Leftrightarrow \\
\displaystyle{ \mathcal{G}_{\mathring{g}}( ( \rho_{R_1}( \mathcal{G}_{\mathring{f}}( \sigma_{A = a} (R').{\bf B} ) )~\kw{as}~fv)\mathop{\Join}_{\substack{ R_1.fv = R.B_i} }  \sigma_{A=a} (R) )}
\Leftrightarrow \\
\displaystyle{ \mathcal{G}_{\mathring{g}}( ( \rho_{R_1}( \mathcal{G}_{\mathring{f}}( \sigma_{A = a} (R').{\bf B} ) )~\kw{as}~fv)\mathop{\Join}_{\substack{ R_1.fv = {\bf B}.B_i} }  \sigma_{A=a} ( \mu_{\bf B}(R') ) )}
\Leftrightarrow \\
\displaystyle{ \mathcal{G}_{\mathring{g}}(  \sigma_{{\bf B}.B_i = \mathcal{G}_{\mathring{f}}( \sigma_{A = a} (R').{\bf B} ) } \mu_{\bf B}(\sigma_{A=a}(R') ) )}
\Leftrightarrow \\
\sigma_{A = a} (\UnnestOp_{{\bf B}}(\Pi_{A, F({\bf B})}(R')))
\end{split}
\end{equation}
where $F({\bf B}) = \mathcal{G}_{\mathring{g}}(\sigma_{B_i = \mathcal{G}_{\mathring{f}}({\bf B})}({\bf B}))$.
}
\comment{
\begin{equation}
% left
\displaystyle{ \sigma_{A = a}( _{A}\mathcal{G}_{\mathring{f}}(R))} 
=
% right
\mathcal{G}_{\mathring{f}}( \sigma_{A = a} (R').{\bf B} )
\label{eq:unnest}
\end{equation}
}
% \end{proof}
